# Supplementary material for: A T-matrix Based Approach to Homogenize Artificial Materials
Source: arXiv:2207.12228 ancillary file (2022-07-25)
Supplement: Supplementary file 1 [file SI.pdf]

# Supplement information: A T-matrix Based Approach to Homogenize Artificial Materials

Benedikt Zerulla,[1] Ramakrishna Venkitakrishnan,[2] Dominik Beutel,[2] Marjan Krstić,[2] Christof Holzer,[2] Carsten Rockstuhl,[1,2] and Ivan Fernandez-Corbaton[1]

[1)] *Institute of Nanotechnology, Karlsruhe Institute of Technology (KIT), D-76344 Eggenstein-Leopoldshafen, Germany*

[2)] *Institute of Theoretical Solid State Physics, Karlsruhe Institute of Technology (KIT), D-76131 Karlsruhe, Germany*

(Dated: 25 July 2022)

## I. ANALYSIS OF LATTICE OF GOLD SPHERES FOR DIFFERENT NUMBERS OF INCLUDED MULTIPOLES

In Sec. 3 of the main text, we consider gold spheres with a radius of $R = 1\,\text{nm}$ placed in a cubic lattice with a lattice constant of $a = 2.05\,\text{nm}$ in a host medium with a relative permittivity of 2.25. In there, the calculations of $\mathbf{T}_{\text{eff}}$ included up to the $N = 5$ multipolar order. In Figure S1(**a**), we observe that the dipolar entry of the effective T-matrix is strongly modified by the interaction with higher order multipoles. We deduce in Figure S1(**b**) that, at the same time, the direct contribution of higher multipoles to the final effective T-matrix is negligible small. Therefore, one can neglect the higher order terms in the effective T-matrix for the homogenization. In Figure S1(**c**), we compare the results for the reflection coefficient for $N = 1$, $N = 3$, and $N = 5$. The predicted response of the material is modified by the incorporation of higher multipoles so that the reflection band appears at longer wavelengths, and a second peak appears for shorter wavelengths. The higher multipoles renormalize the dipoles of the spheres and have to be taken into account. For this example, for which mainly electric multipoles are important, the renormalization of the electric dipoles by multipoles with odd parity is essential. In [1], for instance, it is shown for two-dimensional lattices that electric quadrupoles, in contrast to electric octupoles, do not couple to electric dipoles. The incorporation of multipoles higher than $N = 5$ might slightly shift the reflection band but it also leads to higher numerical errors due to the matrix inversion in Equation (4) as the values of the T-matrix of such small particles related to higher multipolar numbers are very small. We, therefore, truncate the number of included multipoles to $N = 5$. One can deduce from Figure S1(**c**) that the incorporation of higher multipoles than dipoles shifts the spectrum and also leads to a smaller peak for smaller wavelengths. The agreement with the full-wave solver mpGMM is in all cases perfect.

## II. BAND STRUCTURE OF ZN-L-CAMPHORIC ACID-DABCO SURMOF

In Figure S2, the band structure of the Zn-L-camphoric acid-dabco SURMOF analyzed in the main article is displayed. We observe that Bragg resonances do not appear and the material is homogenizable.

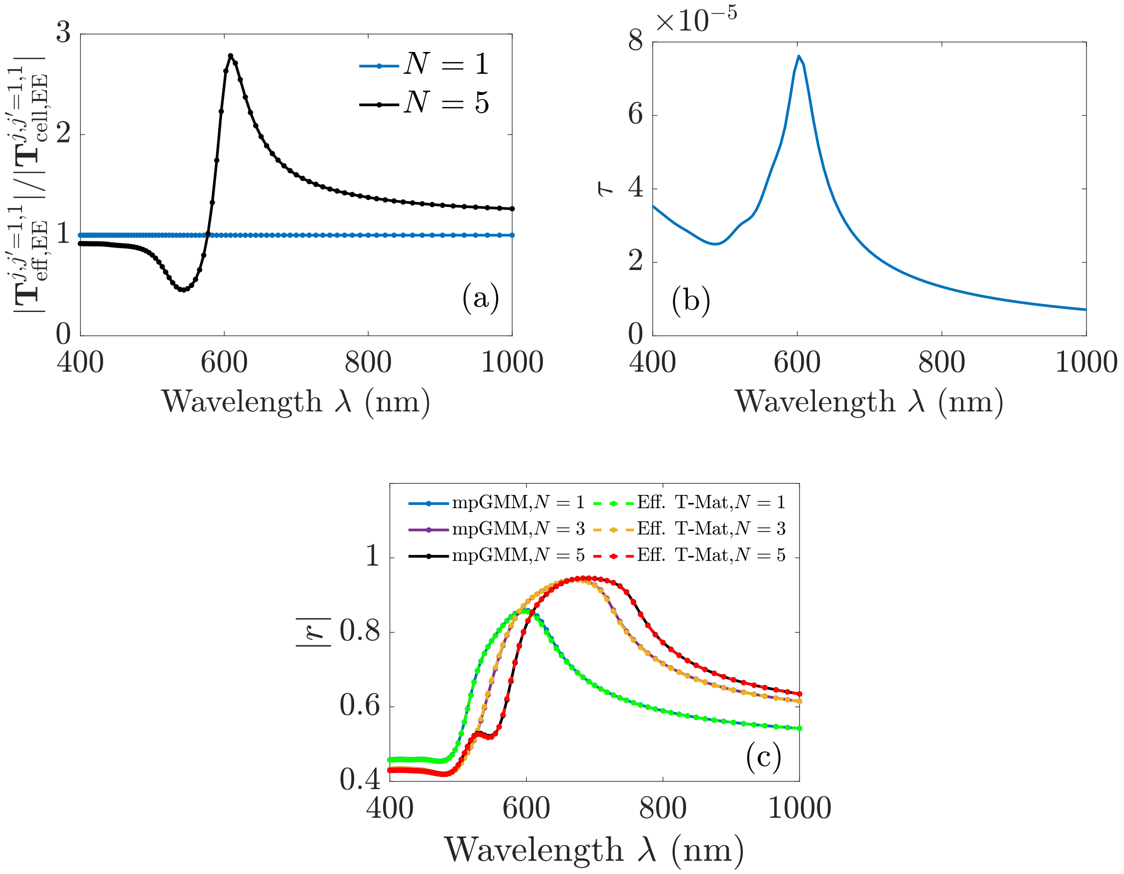


FIG. S1: **(a)** Ratio between the electric dipolar entry of the effective T-matrix of a 3D lattice of gold spheres and the T-matrix of a single isolated sphere when the calculations include only dipoles $N = 1$, or up to $N = 5$ multipoles. **(b)** The dipolar entry is highly modified by the interaction with higher order multipoles inside the lattice. Contribution of higher multipoles to the effective T-matrix. Although the higher multipolar orders influence the dipoles inside the lattice, their final direct contribution in the effective T-matrix is negligible small. The effective dipolar entries alone can be safely used to describe the homogeneous medium. **(c)** Reflection coefficient of a slab of gold spheres. The predicted response of the slab is also significantly modified when higher order multipoles are included in the calculations.

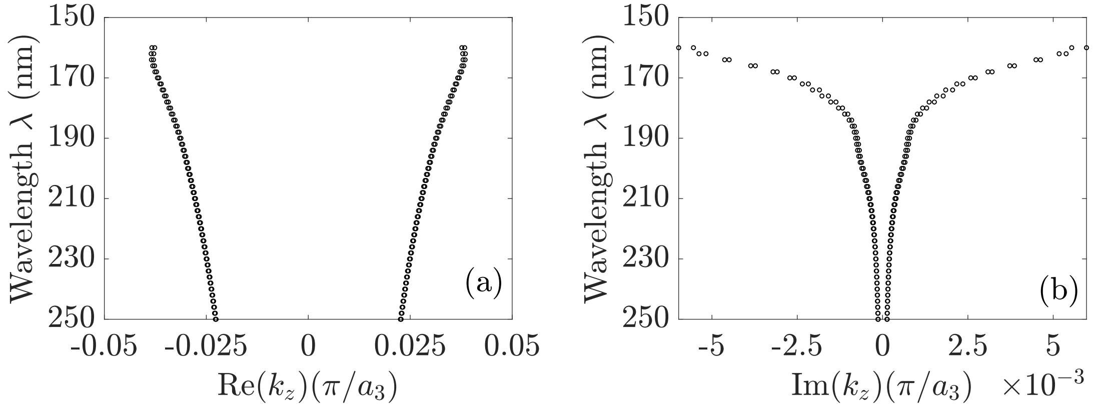


FIG. S2: Band structure of Zn-L-camphoric acid-dabco SURMOF for real **(a)** and imaginary **(b)** propagation constants. Bragg resonances do not appear and the material is homogenizable.

## III. COMPARISON BETWEEN DIFFERENT CALCULATION METHODS OF THE EFFECTIVE T-MATRIX

We show in Figure S3 the comparison between the effective T-matrices $\mathbf{T}_{\text{eff.,Equations}}$ and $\mathbf{T}_{\text{eff.,Analy.}}$ for the example of cut-plate pairs calculated with Equation (3) and with Equation (11) from the main text, respectively. The metric for their difference is defined as

$$\Delta\left(\mathbf{T}_{\text{eff.,Equations}}, \mathbf{T}_{\text{eff.,Analy.}}\right) = \sqrt{\frac{\mathrm{Tr}\left\{\left(\mathbf{T}_{\text{eff.,Equations}} - \mathbf{T}_{\text{eff.,Analy.}}\right)^{\dagger}\left(\mathbf{T}_{\text{eff.,Equations}} - \mathbf{T}_{\text{eff.,Analy.}}\right)\right\}}{2\left(\mathrm{Tr}\left\{\mathbf{T}_{\text{eff.,Equations}}{}^{\dagger}\mathbf{T}_{\text{eff.,Equations}}\right\} + \mathrm{Tr}\left\{\mathbf{T}^{\dagger}_{\text{eff.,Analy.}}\mathbf{T}_{\text{eff.,Analy.}}\right\}\right)}}, \tag{1}$$

so that $\Delta\left(\mathbf{T}_{\text{eff.,Equations}}, \mathbf{T}_{\text{eff.,Analy.}}\right) \in [0,1]$, and a value of 0 means that the two matrices are identical. We observe in Figure S3 that the difference is negligibly small.

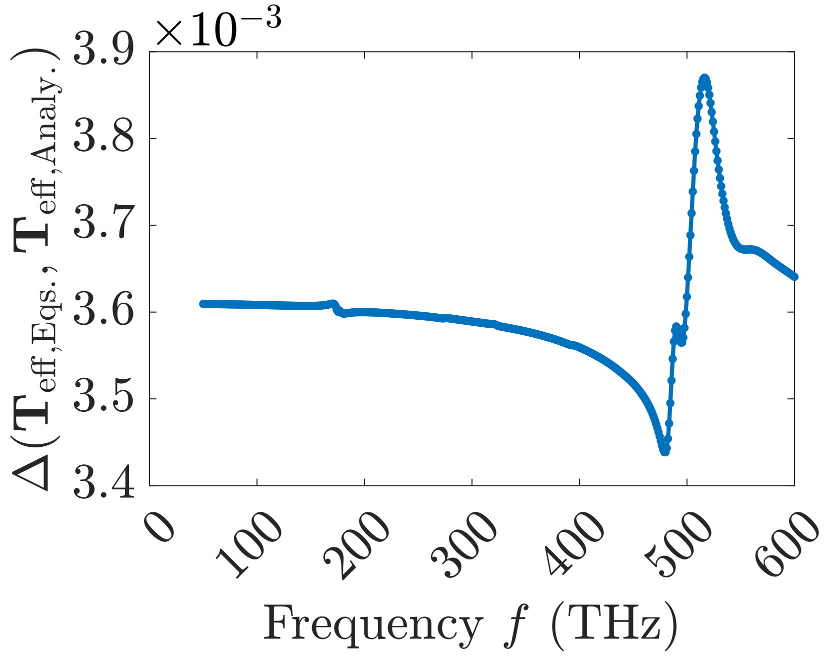


FIG. S3: Normalized difference of effective T-matrices $\mathbf{T}_{\mathrm{eff.,Equations}}$ and $\mathbf{T}_{\mathrm{eff.,Analy.}}$ calculated with Equation (3) and with Equation (11) for the example of cut-plate pairs.

## IV. THE TD-DFT CALCULATIONS OF DYNAMIC POLARIZABILITIES FOR ZN-L-CAMPHORIC ACID-DABCO SURMOF

Complex dynamic polarizability tensors necessary for the construction of the T-matrices of the Zn-L-camphoric acid-dabco SURMOF molecular material for the spectral range of interest were calculated within the time-dependent framework of the density functional theory in development version of the Turbomole code. We used a finite-size molecular cluster-like model cut out of the periodic structure of the Zn-L-camphoric acid-dabco SURMOF and saturated with Hydrogen atoms to properly coordinate broken bonds at the edge of the periodic lattice. The full $6 \times 6$ polarizability tensors were calculated for discreet wavelengths for every 2 nm from 160-350 nm. These polarizaility tensors are equivalent to the dipolar T-matrix [2]. We used the Coulomb-attenuating long-range corrected CAM-B3LYP functional [3] together with a def2-SVP basis set [4]. The same Coulomb fitting basis set was used [5]. The damping factor was set to 0.25 eV at half-width at half-maximum. Additionally, the resolution of identity (RI) algorithm [6] with multipole accelerated RI-J and semi-numerical exchange [7] to speed up the calculations were employed. Magnetic-magnetic dynamic polarizabilities were calculated with Gauge-Including

Atomic Orbitals (GIAO). The dynamic polarizabilities were used to construct $\mathbf{T}_{\text{cell}}$.

## REFERENCES


[1] A. Rahimzadegan, T. D. Karamanos, R. Alaee, A. G. Lamprianidis, D. Beutel, R. W. Boyd, and C. Rockstuhl, "A comprehensive multipolar theory for periodic metasurfaces," *Adv. Opt. Mater.* **10**, 2102059 (2022).

[2] I. Fernandez-Corbaton, D. Beutel, C. Rockstuhl, A. Pausch, and W. Klopper, "Computation of electromagnetic properties of molecular ensembles," *ChemPhysChem* **21**, 878–887 (2020).

[3] T. Yanai, D. P. Tew, and N. C. Handy, "A new hybrid exchange–correlation functional using the coulomb-attenuating method (cam-b3lyp)," *Chem. Phys. Lett.* **393**, 51–57 (2004).

[4] F. Weigend and R. Ahlrichs, "Balanced basis sets of split valence, triple zeta valence and quadruple zeta valence quality for h to rn: Design and assessment of accuracy," *Phys. Chem. Chem. Phys.* **7**, 3297–3305 (2005).

[5] F. Weigend, "Accurate coulomb-fitting basis sets for h to rn," *Phys. Chem. Chem. Phys.* **8**, 1057–1065 (2006).

[6] R. Bauernschmitt, M. Häser, O. Treutler, and R. Ahlrichs, "Calculation of excitation energies within time-dependent density functional theory using auxiliary basis set expansions," *Chem. Phys. Lett.* **264**, 573–578 (1997).

[7] C. Holzer, "An improved seminumerical coulomb and exchange algorithm for properties and excited states in modern density functional theory," *J. Chem. Phys.* **153**, 184115 (2020).
